# Supplementary material for: Evaluating and Advancing Multimodal Large Language Models in Perception Ability Lens
Source: arXiv:2411.14725 source file (2025-06-03)
Supplement: Supplementary file 1 [file X_suppl.tex]

% \setcounter{page}{1}
% \maketitlesupplementary

%In this supplementary material, we provide: (1) implementation details, and (2) benchmark analysis.

\section{Implementation Details}
We implement LLaVA-OV-SI following the methodology outlined in ~\cite{llava-ov}. The training process consists of three stages: language-image alignment (Stage 1), high-quality knowledge learning (Stage 1.5 or MID stage), and single-image visual instruction tuning (SI stage). We utilize the same dataset as LLaVA-OV with minor differences, as a portion of the single-image dataset has not yet been released. The final results are comparable to the official checkpoint of LLaVA-OV-SI, as demonstrated in Table \ref{tab total}. To investigate the universality of the observed ability conflicts, we replace the LLM of LLaVA-OV-SI with Phi3.5-3.8b~\cite{phi3} and Gemma2-2b~\cite{gemma},  replace the visual encoder with CLIP-Large~\cite{clip}, and adjust the data ratio while keeping the other training configurations unchanged.

\section{Analyzing the AbilityLens}
%\section{More details of the AbilityLens}

\noindent \textbf{Ability selection.} We select six perception abilities based on the following principles:

\begin{itemize}
    \item The abilities should encompass different levels of image perception granularity, such as entities (image level), grounding (region level), and OCR (pixel level).
    \item They should capture the ability to perceive and understand diverse types of data. Therefore, we include structured data, which spans charts, graphs, code, posters, maps, and diagrams.
    \item While primarily a perception-centric benchmark, the abilities should also demonstrate a basic level of reasoning based on perceived signals. For instance, locating an object and recognizing its attributes.
\end{itemize}

Considering these factors, we propose the following six abilities: counting, OCR, attribute recognition, entity extraction, grounding, and structural data understanding.

\noindent \textbf{Ability confusion matrix.} We  present the ability correlation matrix in Figure \ref{fig ability}. The results indicate that OCR exhibits low correlation with other abilities, whereas entity recognition and counting show a strong correlation. Similarly, grounding and structured data understanding also display a strong correlation.

\noindent \textbf{Selected MLLM benchmark performance confusion matrix.} We evaluate the sub-metrics of selected benchmarks using 14 MLLMs and present the results as a correlation matrix. As illustrated in Figure \ref{fig: benchmark}, the findings indicate significant performance variance across different domains, metrics, and question types within the benchmarks.

\section{More Results}

As shown in Figure~\ref{fig encoder}, we examine the impact of the visual encoder on ability conflicts. We observe that SigLIP and CLIP-L exhibit similar performance trends during training, suggesting that the encoder is not the primary cause of ability conflict. Additional results analyzing the effects of the LLM and training data are presented in Figures 5 and 6 of our paper.

\begin{figure}[t]
    \centering
    \includegraphics[width=1\linewidth]{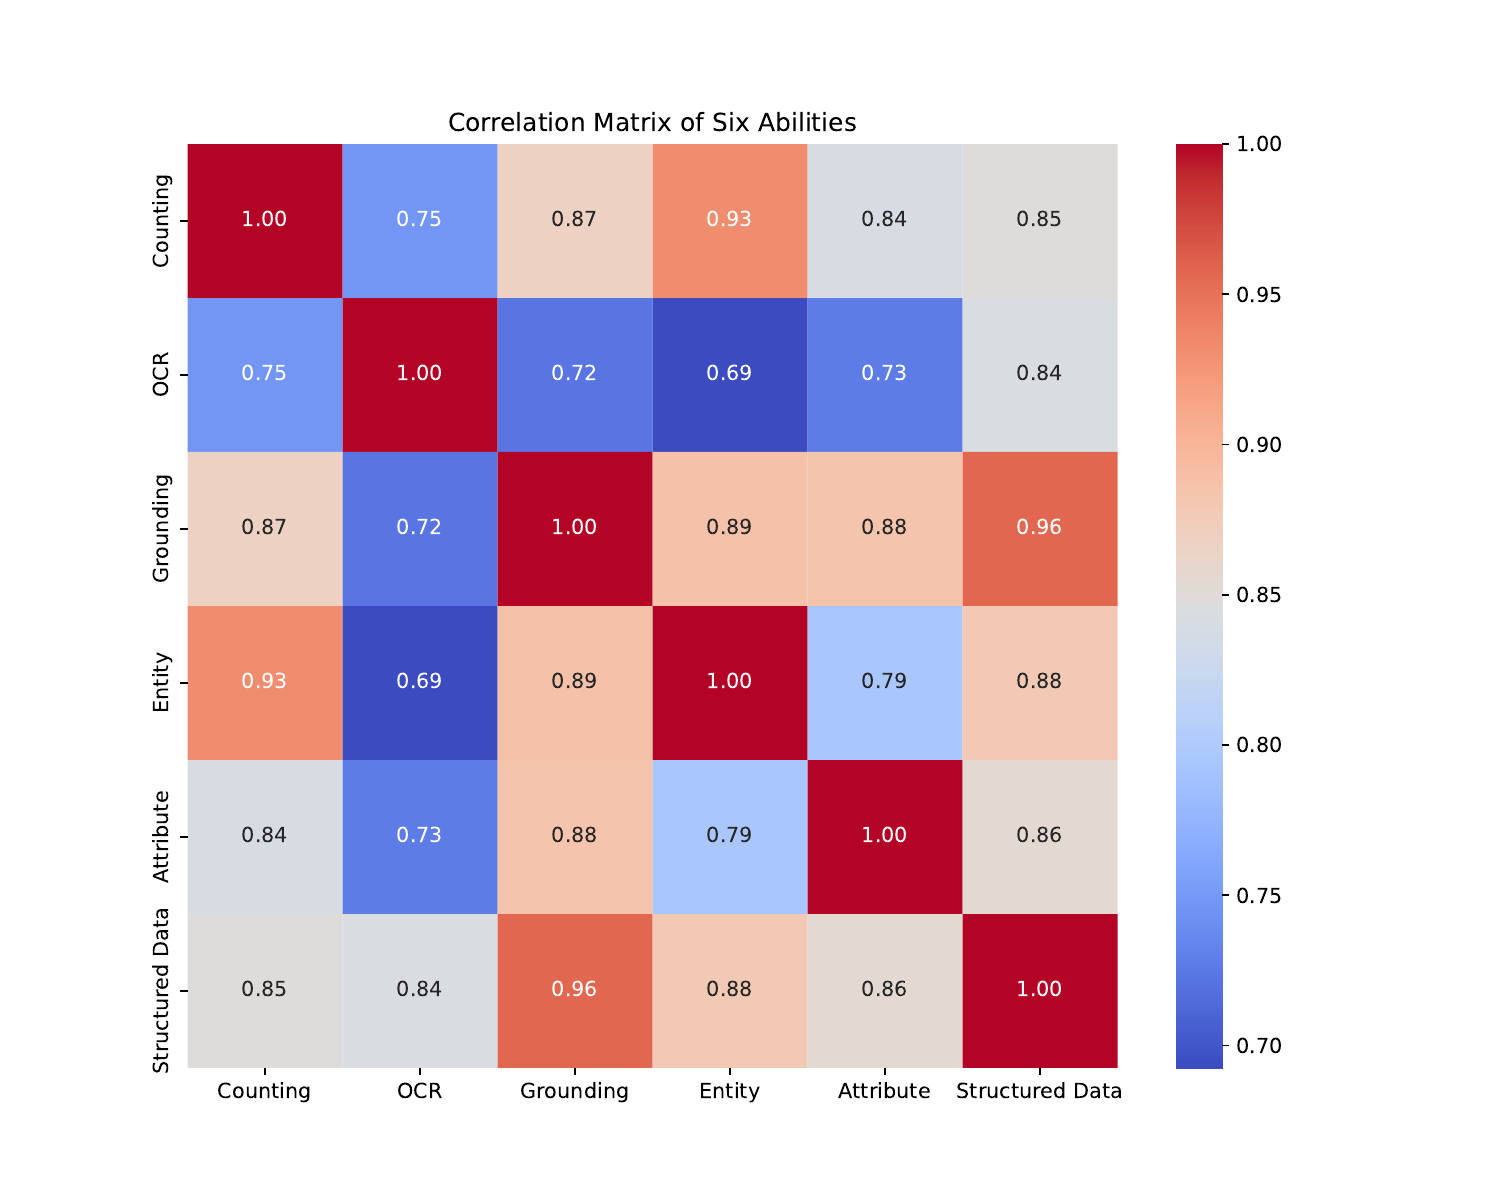}
    \caption{Pearson correlation matrix between six abilities with respect to 14 MLLMs. The correlation matrix helps us to analysis and group different kinds of data.}
    \label{fig ability}
\end{figure}

\begin{figure*}
    \centering
    \includegraphics[width=0.8\linewidth]{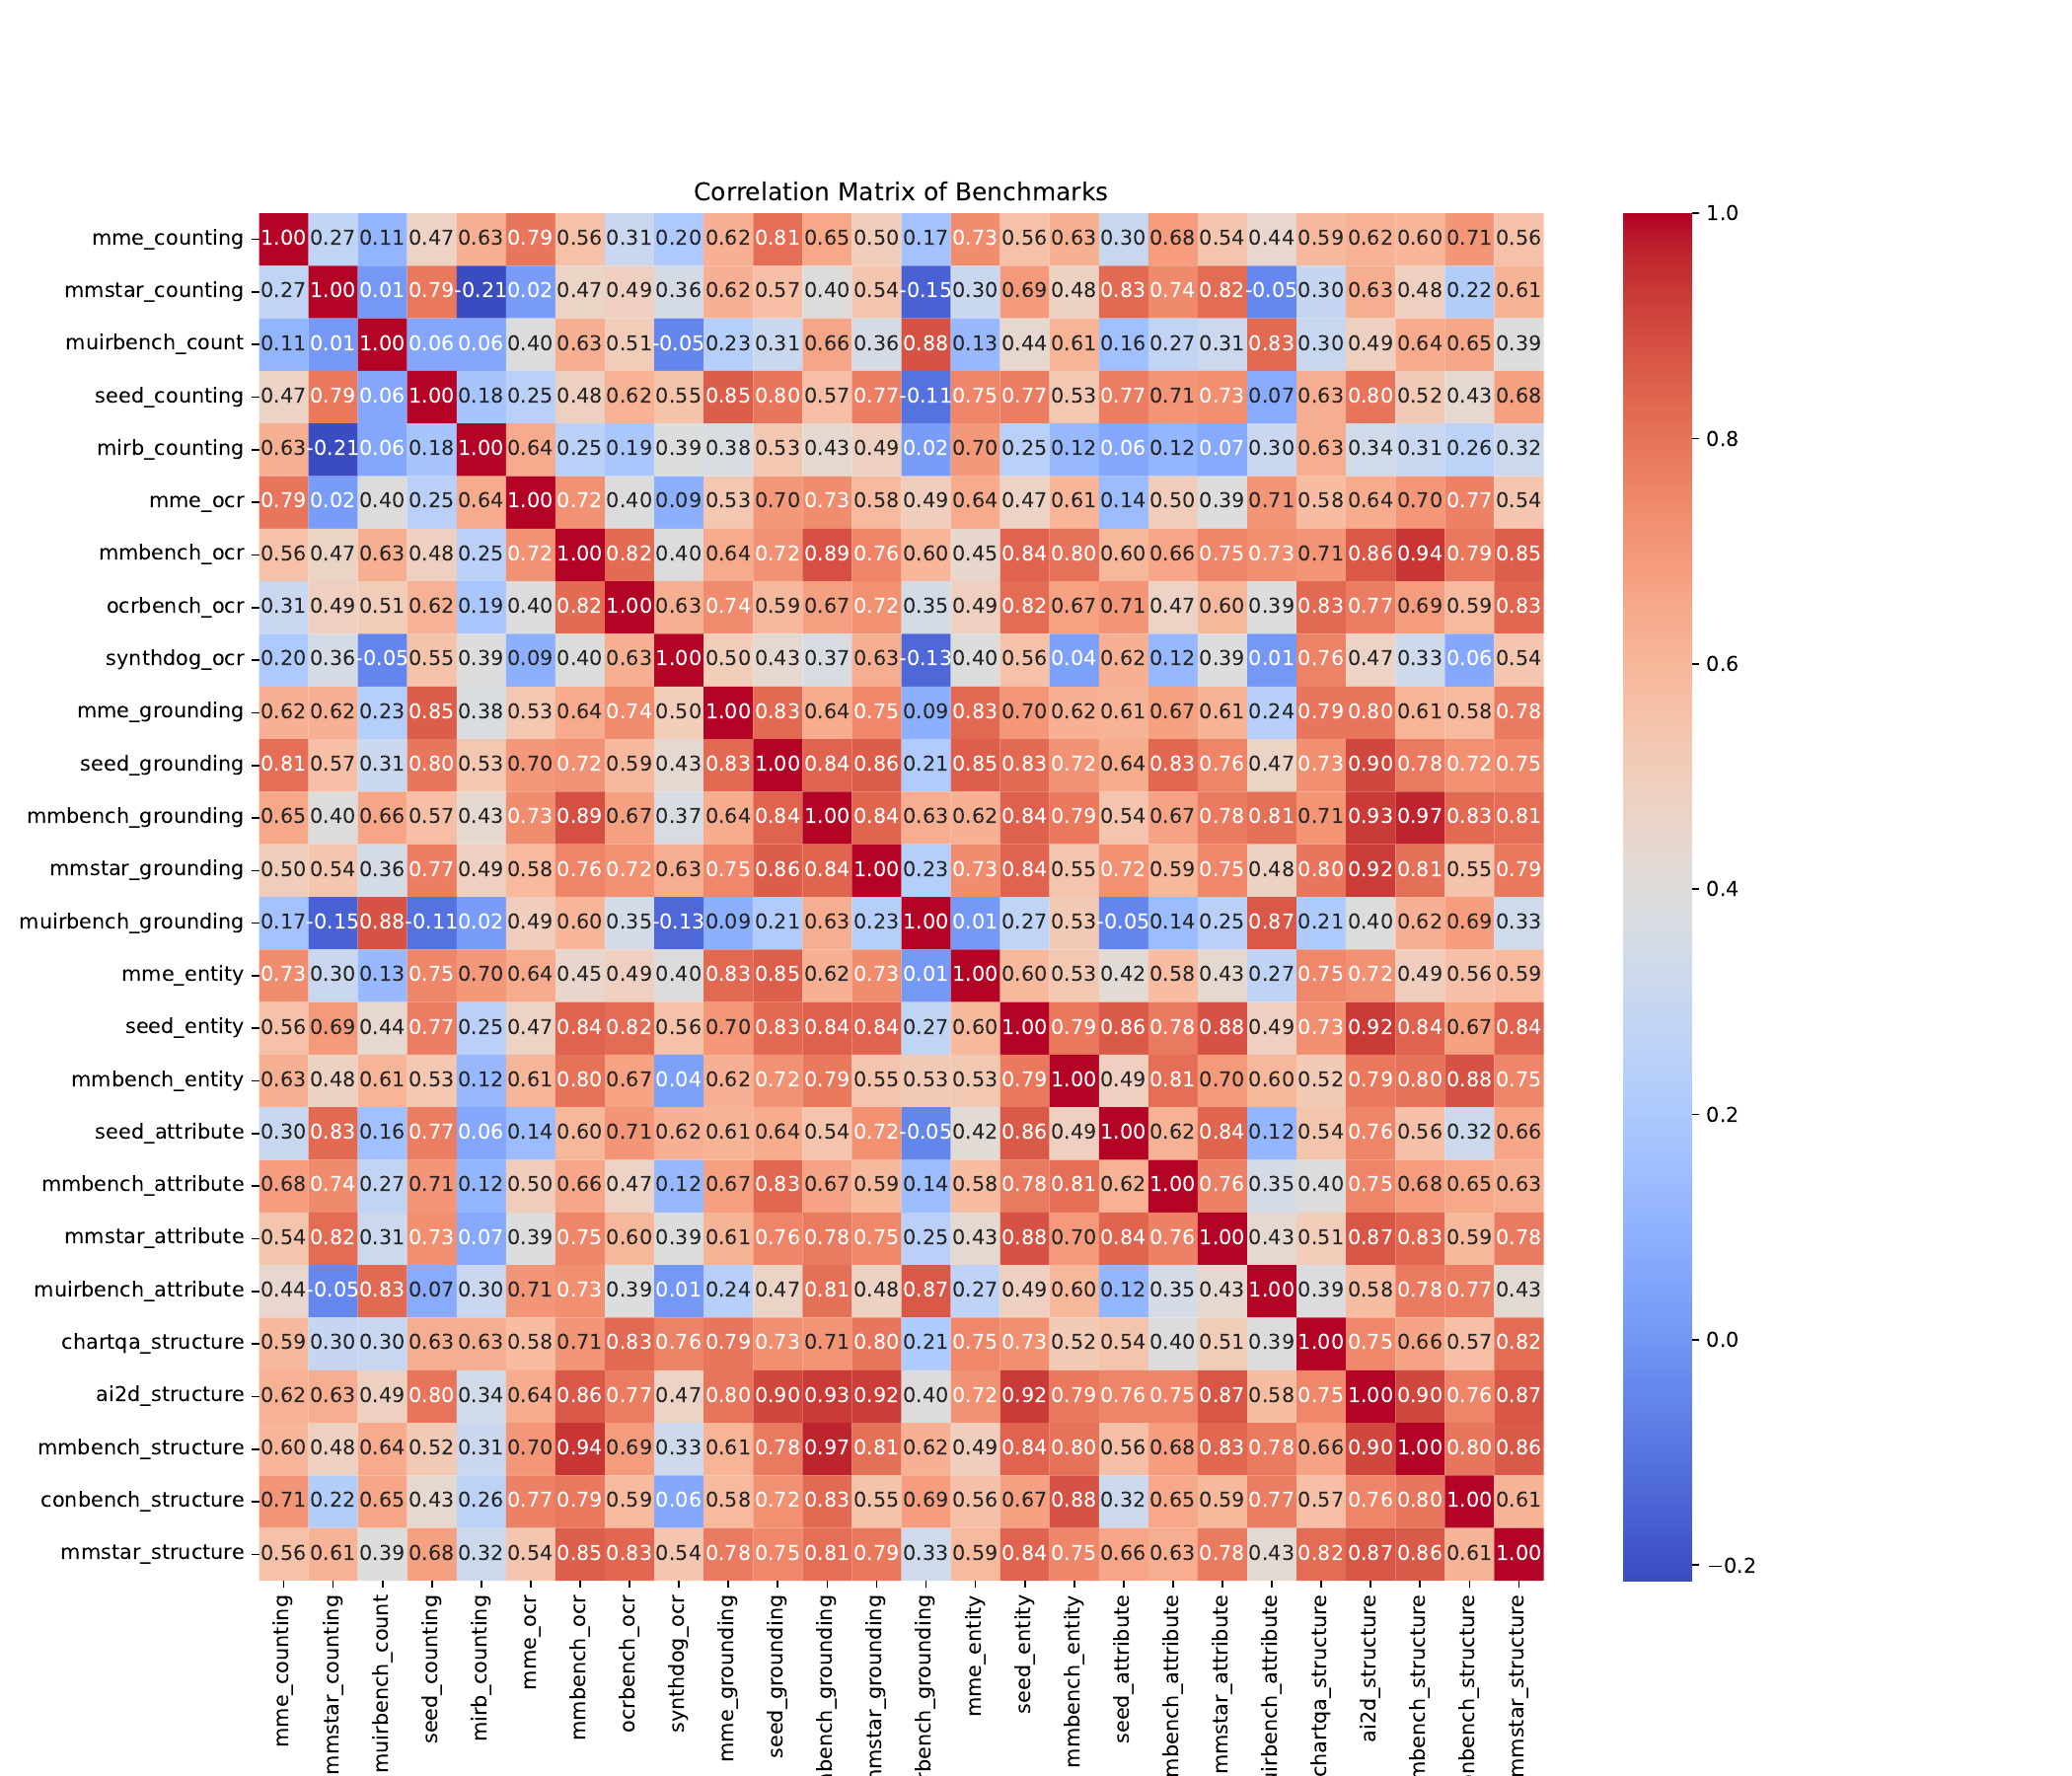}
    \caption{Pearson correlation matrix for selected MLLM benchmarks with respect to 14 MLLMs.}
    \label{fig: benchmark}
\end{figure*}

\begin{figure*}[htbp]
    \centering
    % 第一子图
    \begin{subfigure}[b]{\textwidth} % 设置子图宽度
        \centering
        \includegraphics[width=1.05\textwidth]{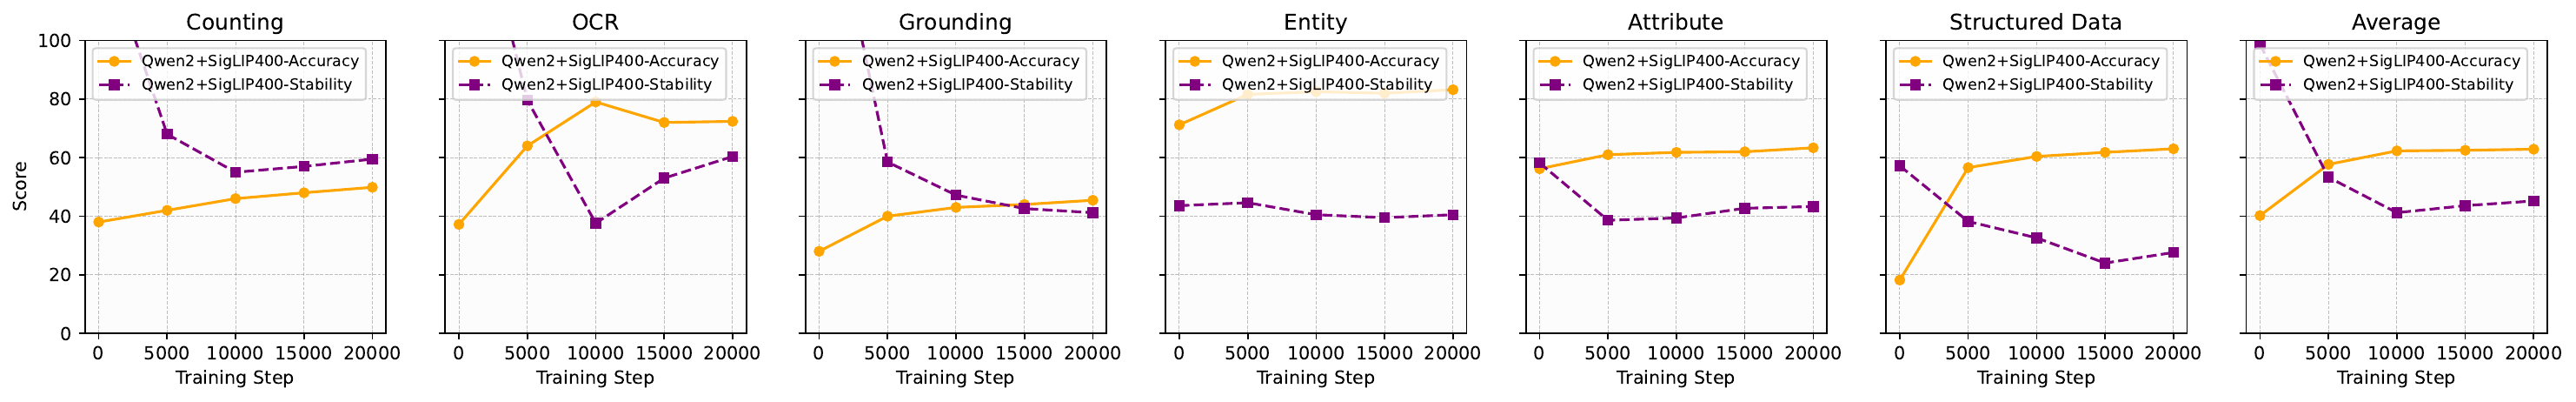}
        \label{fig:subfig1}
    \end{subfigure}

    % 第二子图
    \begin{subfigure}[b]{\textwidth}
        \centering
        \includegraphics[width=1.05\textwidth]{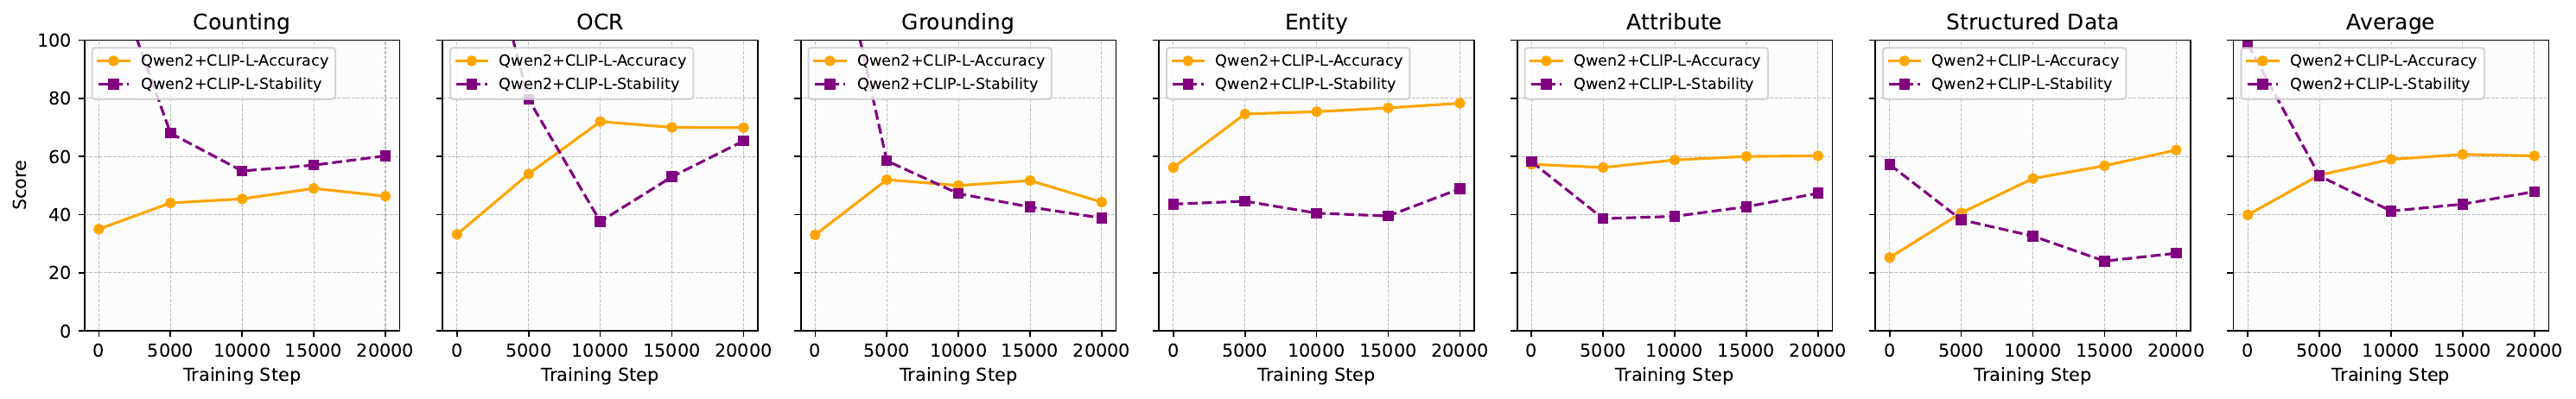}
        \label{fig:subfig2}
    \end{subfigure}

    \caption{Monitoring the training dynamics of LLaVA-OV-SI-Qwen2-7b using CLIP-Large (first row) and SigLIP400m (second row) across six abilities.}
    \label{fig encoder}
\end{figure*}

% \begin{figure*}[htbp]
%     \centering
%     % 第一子图
%     \begin{subfigure}[b]{\textwidth} % 设置子图宽度
%         \centering
%         \includegraphics[width=1.05\textwidth]{ICCV2025-Author-Kit-Feb/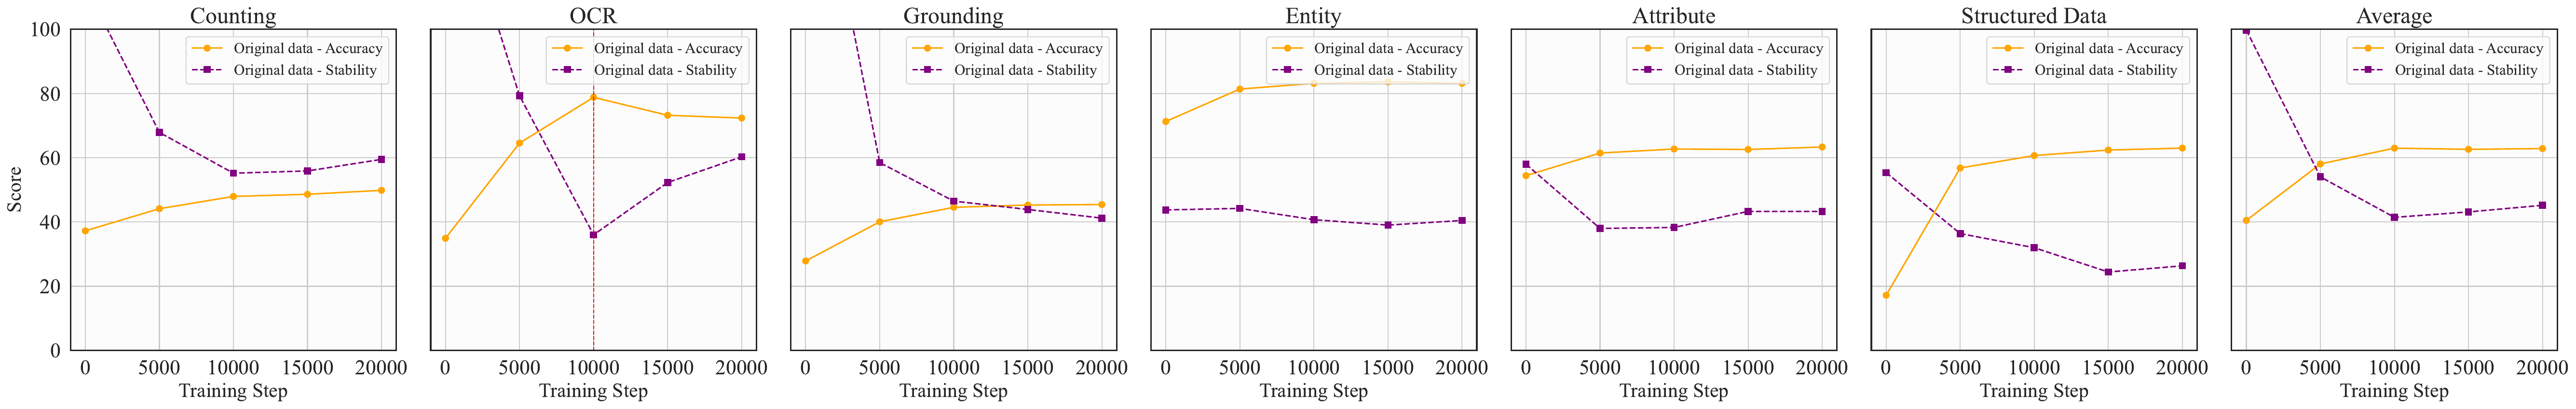}
%         \label{fig:subfig1}
%     \end{subfigure}

%     % 第二子图
%     \begin{subfigure}[b]{\textwidth}
%         \centering
%         \includegraphics[width=1.05\textwidth]{ICCV2025-Author-Kit-Feb/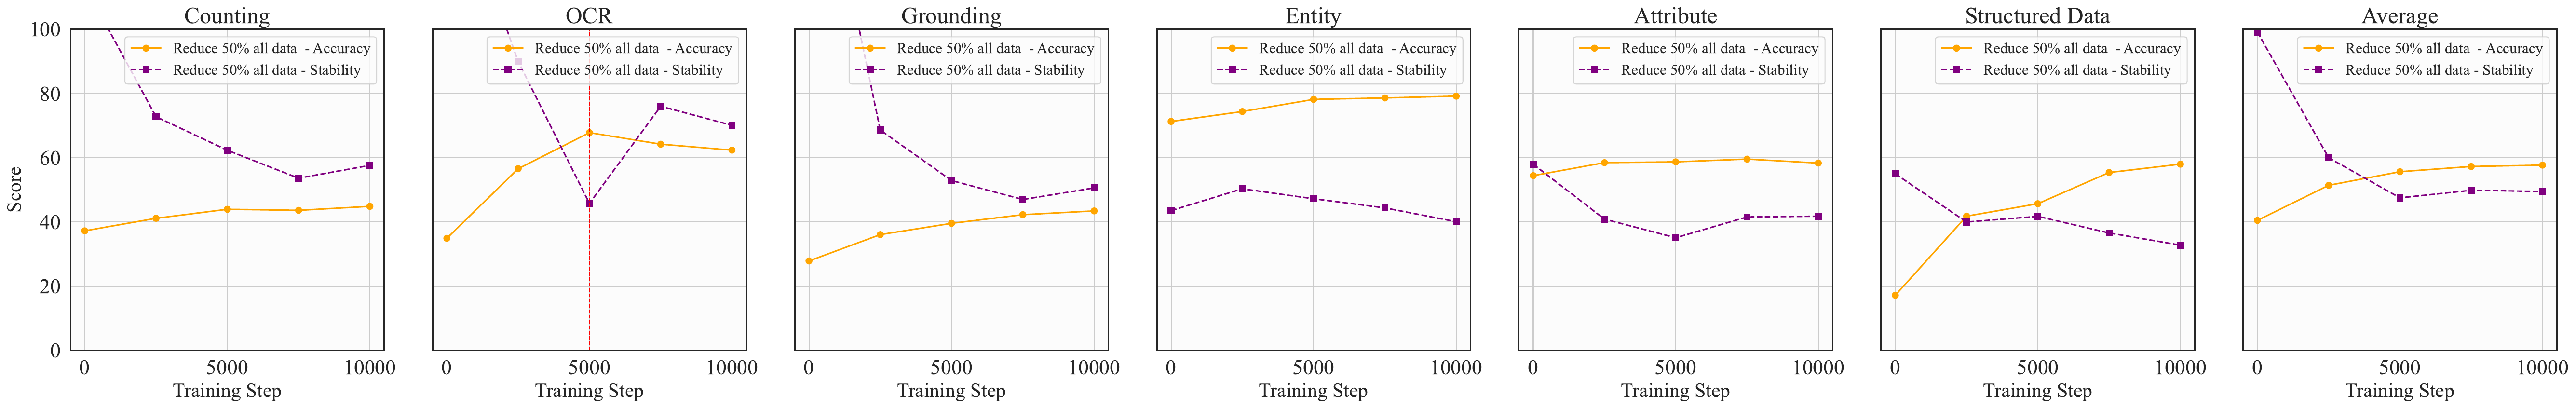}
%         \label{fig:subfig2}
%     \end{subfigure}

%     % 第三子图
%     \begin{subfigure}[b]{\textwidth}
%         \centering
%         \includegraphics[width=1.05\textwidth]{ICCV2025-Author-Kit-Feb/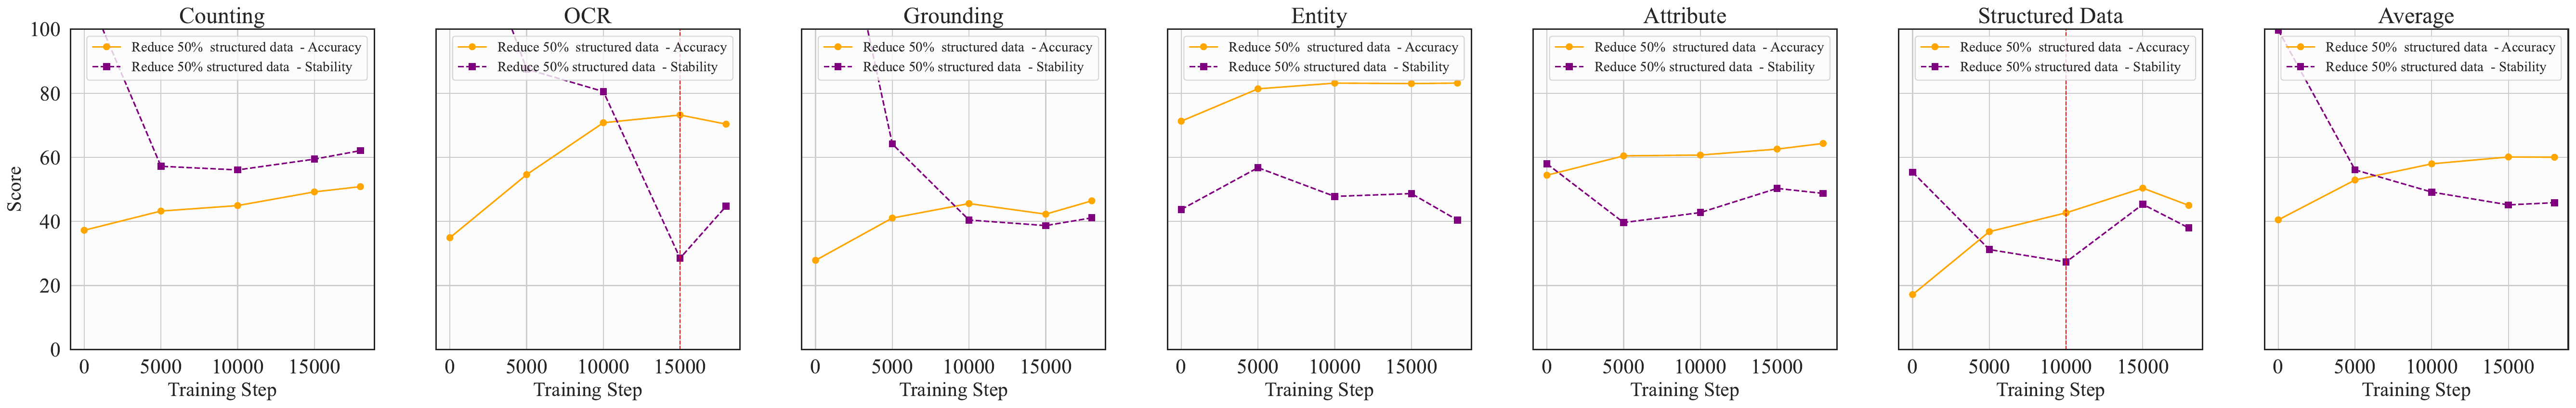}
%         \label{fig:subfig3}
%     \end{subfigure}

%     \caption{Monitoring the training dynamics of LLaVA-OV-SI using original data (first row), 50\% original data (second row), and data reducing 50\% structured data (third row) across six abilities. }
%     \label{fig data}
% \end{figure*}

\begin{table*}[h]\caption{Results of reimplemented LLaVA-OV-SI with different LLMs and using ASMM to alleviate ability conflict. We use 10 representative benchmarks including AI2D~\cite{ai2d}, MMBench~\cite{MMBench}, MME~\cite{mme}, SeedBench~\cite{seedbench}, ScienceQA~\cite{scienceqa}, RealWorldQA~\cite{realwordqa}, ChartQA~\cite{masry2022chartqa}, DocVQA~\cite{docvqa}, InfoVQA~\cite{infovqa}, and MMStar~\cite{mmstar} where ScienceQA and RealWorldQA are abbreviated to S-QA and RWQA. $\dagger$ indicates that the model was obtained through reimplementation.}
\centering
\resizebox{\linewidth}{!}{
\begin{tabular}{lcccccccccccc}
\toprule
\textbf{Model} & \textbf{SUM} & \textbf{AVG} & \textbf{AI2D} & \textbf{MMBench} & \textbf{MME} & \textbf{SeedBench} & \textbf{S-QA} & \textbf{RWQA} & \textbf{ChartQA} & \textbf{DocVQA(val)} & \textbf{InfoVQA(val)} & \textbf{MMStar} \\
\hline
Qwen2-7b(official)         & 774.4 & 77.4 & 81.6 & 81.7 & 2109 & 74.8 & 96.6 & 65.5 & 78.8 & 89.3 & 69.9 & 60.9 \\
Qwen2-7b$\dagger$         & 768.7 & 76.9 & 79.0 & 80.3 & 2030 & 73.2 & 96.1 & 67.0 & 81.6 & 91.2 & 70.6 & 57.3 \\
Phi3.5-3.8b$\dagger$       & 664.6 & 66.5 & 73.6 & 77.8 & 1719 & 71.3 & 96.1 & 55.0 & 66.2 & 65.3 & 47.9 & 50.0 \\
Gemma2-2b$\dagger$         & 663.7 & 66.4 & 71.7 & 76.0 & 1703 & 70.8 & 94.0 & 57.1 & 68.6 & 68.7 & 47.8 & 48.1 \\
\bottomrule
\end{tabular}}
\label{tab total}
\end{table*}
